# Supplementary material for: 4D Spatio-Temporal ConvNets: Minkowski Convolutional Neural Networks
Source: arXiv:1904.08755 source file (2019-06-13)
Supplement: Supplementary file 1 [file supplementary.pdf]

# The supplementary material for 4D Spatio-Temporal ConvNets: Minkowski Convolutional Neural Networks

## 1. Minkowski Engine

In this section, we provide detailed breakdowns of few algorithms in the main paper as well as the coordinate initialization and the hash function. Please note that the actual implementation may not faithfully reflect the algorithms presented here for optimization.

### 1.1. Sparse Quantization

First, we provide line-by-line comments for the sparse quantization algorithm. Overall, the algorithm finds unique voxels and creates labels associated with them. If there are different labels within the same voxel, we assign the `IGNORE_LABEL`. This allows the network to ignore the cross-entropy loss for those voxels during training.

The Alg. 1 starts by converting all coordinates to hash keys and generating a sequence $\mathbf{i}$, which is used to identify the original indices. Next, we sort the sequence, label pairs by the hash key (L5). This will place indices and labels that fall into the same cell to be adjacent in the GPU memory. Next, we reduce the index sequence with the key-label pair (L6). This step will collapse all points with the same labels. However, if there are different labels within the same cell, we will have at least two key-label pairs in the same cell. Thus, in L7, we use the reduction function $f((l_x, i_x), (l_y, i_y)) => (\texttt{IGNORE\_LABEL}, i_x)$ will simply assign `IGNORE_LABEL` to the cell. Finally, we use the reduced unique indices $\mathbf{i}'''$ to return unique coordinates, features, and transformed labels.

**Algorithm 1** GPU Sparse Tensor Quantization

1: Inputs: coordinates $C_p \in \mathbb{R}^{N \times D}$, features $F_p \in \mathbb{R}^{N \times N_f}$, target labels $\mathbf{l} \in \mathbb{Z}_+^N$, quantization step size $v_l$
2: $C'_p \leftarrow$ floor($C_p$ / $v_l$)
3: $\mathbf{k} \leftarrow$ hash($C'_p$)
4: $\mathbf{i} \leftarrow$ sequence(N)
5: $((\mathbf{i}', \mathbf{l}'), k') \leftarrow$ SortByKey($(\mathbf{i}, \mathbf{l})$, key=$\mathbf{k}$)
6: $(\mathbf{i}'', (\mathbf{k}'', \mathbf{l}'')) \leftarrow$ UniqueByKey($\mathbf{i}'$, key=$(\mathbf{k}', \mathbf{l}')$)
7: $(\mathbf{l}''', \mathbf{i}''') \leftarrow$ ReduceByKey($(\mathbf{l}'', \mathbf{i}'')$, key=$\mathbf{k}''$, fn=$f$)
8: **return** $C'_p[\mathbf{i}''', :], F_p[\mathbf{i}''', :], \mathbf{l}'''$

### 1.2. Coordinate Hashing

We used a variation of Fowler–Noll–Vo hash function, *FNV64-1A*, and modified it for coordinates in `int32`. We list the algorithm in Alg. 2.

### 1.3. Creating output coordinates

The first step in the generalized sparse convolution is defining the output coordinates $\mathcal{C}^{\text{out}}$. In most cases, we use the same coordinates for the output coordinates. However, when we use a strided convolution or a strided pooling, we use the Alg. 3 to create new output coordinates. For transposed strided convolutions, we use the same coordinates with the same input-stride to preserve the order of the coordinates.

**Algorithm 2** Coordinate Hashing

**Require:** Inputs: coordinate $\mathbf{c} \in \mathbb{Z}^D$ in `int32`
**function** HASH($\mathbf{c}$)
  $h$ = UINT64(14695981039346656037)
  **for all** $\mathbf{c}_i \in \mathbf{c}$ **do**
    $h = h \oplus$ UINT32($c_i$)
    $h = h \times$ UINT64(1099511628211)
  **end for**
  **return** $h$
**end function**

**Algorithm 3** Create output coordinates

**Require:** input stride $s_i$, layer stride $s_l$, input coordinates $\mathbf{C}$
**function** CREATEOUTPUTCOORDINATES($\mathbf{C}$, $s_i$, $s_l$)
  **if** $s_l > 1$ **then**
    $s \leftarrow s_l \times s_i$
    $\mathbf{C}' \leftarrow \{\}$ // Create an empty set
    **for all** $\mathbf{c}_i \in \mathbf{C}$ **do**
      $\mathbf{c} \leftarrow \lfloor \mathbf{c}_i / s \rfloor \times s$
      **if** $\mathbf{c}$ is not in $\mathbf{C}'$ **then**
        Append $\mathbf{c}$ to $\mathbf{C}'$
      **end if**
    **end for**
    **return** $\mathbf{C}'$
  **else**
    **return** $\mathbf{C}$
  **end if**
**end function**

## 2. Derivation of the Trilateral Stationary-Conditional Random Field Fixed Point Update Equation

The TS-CRF optimization $\arg\max_{\mathbf{X}} P(X)$ is intractable. Instead, we use the variational inference to minimize divergence between the optimal $P(\mathbf{X})$ and an approximated distribution $Q(\mathbf{X})$. Commonly, the divergence is measured using the I-projection: $\mathbf{D}(Q\|P)$, the number of bits lost when coding a distribution $Q$ using $P$. To simplify the approximated distribution, we use the mean-field approximation, $Q = \prod_i Q_i(x_i)$ as the closed form solution exists. From the Theorem 11.9 in [4], $Q$ is a local maximum if and only if

$$Q_i(x_i) = \frac{1}{Z_i} \exp \mathop{\mathbf{E}}_{\mathbf{X}_{-i} \sim Q_{-i}} \left[ \phi_u(x_i) + \sum_{j \in \mathcal{N}(x_i)} \phi_p(x_i, x_j) \right] \tag{1}$$

. where $\mathbf{X}_{-i}$ and $Q_{-i}$ indicate all variables except for the $i$-th variable.

$$Q_i(x_i) = \frac{1}{Z_i} \exp \mathop{\mathbf{E}}_{\mathbf{X}_{-i} \sim Q_{-i}} \left[ \phi_u(x_i) + \sum_{j \in \mathcal{N}(x_i)} \phi_p(x_i, x_j) \right] \tag{2}$$

$$= \frac{1}{Z_i} \exp \left[ \mathop{\mathbf{E}}_{\mathbf{X}_{-i} \sim Q_{-i}} \phi_u(x_i) + \mathop{\mathbf{E}}_{\mathbf{X}_{-i} \sim Q_{-i}} \sum_{j \in \mathcal{N}(x_i)} \phi_p(x_i, x_j) \right] \tag{3}$$

$$= \frac{1}{Z_i} \exp \left[ \phi_u(x_i) + \sum_{j \in \mathcal{N}(x_i)} \mathbf{E}_{j \in \mathcal{N}(x_i)} \phi_p(x_i, x_j) \right] \tag{4}$$

$$= \frac{1}{Z_i} \exp \left[ \phi_u(x_i) + \sum_{j \in \mathcal{N}(x_i)} \sum_{x_j} \phi_p(x_i, x_j) Q_j(x_j) \right] \tag{5}$$

Thus, the final fixed-point update equation is

$$Q_i^+(x_i) = \frac{1}{Z_i} \exp \left\{ \phi_u(x_i) + \sum_{j \in \mathcal{N}(x_i)} \sum_{x_j} \phi_p(x_i, x_j) Q_j(x_j) \right\} \tag{6}$$

.

# 3. Experiments and Analysis

We present per-class IoU numbers for all experiments and more qualitative results. We also visualize the entire RueMongue 2014 (Varcity) dataset on Fig. 1. The dataset is quite small for deep learning so the Minkowski Networks results are all saturated around 66% mIoU.

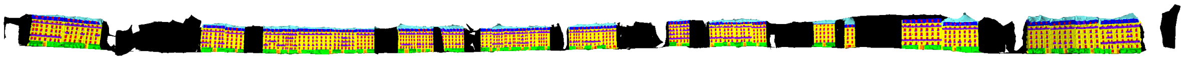

Figure 1: Visualization of the RueMonge 2014 dataset ground-truth. The left half of the pointcloud is the training set and the right half is the test set (Black: `IGNORE_LABEL`).

Table 1: ScanNet [1] 3D Segmentation Benchmark Results

| Method | bath | bed | bksf | cab | chair | cntr | curt | desk | door | floor | othr | pic | ref | show | sink | sofa | tab | toil | wall | wind | **mIoU** |
|---|---|---|---|---|---|---|---|---|---|---|---|---|---|---|---|---|---|---|---|---|---|
| ScanNet [1] | 20.3 | 36.6 | 50.1 | 31.1 | 52.4 | 21.1 | 0.2 | 34.2 | 18.9 | 78.6 | 14.5 | 10.2 | 24.5 | 15.2 | 31.8 | 34.8 | 30.0 | 46.0 | 43.7 | 18.2 | 30.6 |
| SSC-UNet [3] | 35.3 | 29.0 | 27.8 | 16.6 | 55.3 | 16.9 | 28.6 | 14.7 | 14.8 | 90.8 | 18.2 | 6.4 | 2.3 | 1.8 | 35.4 | 36.3 | 34.5 | 54.6 | 68.5 | 27.8 | 30.8 |
| PointNet++ [9] | 58.4 | 47.8 | 45.8 | 25.6 | 36.0 | 25.0 | 24.7 | 27.8 | 26.1 | 67.7 | 18.3 | 11.7 | 21.2 | 14.5 | 36.4 | 34.6 | 23.2 | 54.8 | 52.3 | 25.2 | 33.9 |
| ScanNet+SDF | 29.7 | 49.1 | 43.2 | 35.8 | 61.2 | 27.4 | 11.6 | 41.1 | 26.5 | 90.4 | 22.9 | 7.9 | 25.0 | 18.5 | 32.0 | 51.0 | 38.5 | 54.8 | 59.7 | 39.4 | 38.3 |
| SPLATNet [11] | 47.2 | 51.1 | 60.6 | 31.1 | 65.6 | 24.5 | 40.5 | 32.8 | 19.7 | 92.7 | 22.7 | 0.0 | 0.1 | 24.9 | 27.1 | 51.0 | 38.3 | 59.3 | 69.9 | 26.7 | 39.3 |
| TangetConv [12] | 43.7 | 64.6 | 47.4 | 36.9 | 64.5 | 35.3 | 25.8 | 28.2 | 27.9 | 91.8 | 29.8 | 14.7 | 28.3 | 29.4 | 48.7 | 56.2 | 42.7 | 61.9 | 63.3 | 35.2 | 43.8 |
| SurfaceConv [7] | 50.5 | 62.2 | 38.0 | 34.2 | 65.4 | 22.7 | 39.7 | 36.7 | 27.6 | 92.4 | 24.0 | 19.8 | 35.9 | 26.2 | 36.6 | 58.1 | 43.5 | 64.0 | 66.8 | 39.8 | 44.2 |
| 3DMV [2] | 48.4 | 53.8 | 64.3 | 42.4 | 60.6 | 31.0 | 57.4 | 43.3 | 37.8 | 79.6 | 30.1 | 21.4 | 53.7 | 20.8 | 47.2 | 50.7 | 41.3 | 69.3 | 60.2 | 53.9 | 48.4 |
| 3DMV-FTSDF | 55.8 | 60.8 | 42.4 | 47.8 | 69.0 | 24.6 | 58.6 | 46.8 | 45.0 | 91.1 | 39.4 | 16.0 | 43.8 | 21.2 | 43.2 | 54.1 | 47.5 | 74.2 | 72.7 | 47.7 | 50.1 |
| MinkowskiNet42 (5cm) | 81.1 | 73.4 | 73.9 | 64.1 | 80.4 | 41.3 | 75.9 | 69.6 | 54.5 | 93.8 | 51.8 | 14.1 | 62.3 | 75.7 | 68.0 | 72.3 | 68.4 | 89.6 | 82.1 | 65.1 | 67.9 |
| MinkowskiNet42 (2cm) | 83.7 | 80.4 | 80.0 | 72.1 | 84.3 | 46.0 | 83.5 | 64.7 | 59.7 | 95.3 | 54.2 | 21.4 | 74.6 | 91.2 | 70.5 | 77.1 | 64.0 | 87.6 | 84.2 | 67.2 | 72.1 |

Test labels not available publicly. All numbers from `http://kaldir.vc.in.tum.de/scannet_benchmark/`. Entries without citation are from unpublished works. ‡: uses 2D images additionally.

Table 2: Results on the Stanford 3D Indoor Spaces Dataset Area 5 Test (Fold #1) (S3DIS)

| Method | ceiling | floor | wall | beam | clmn | windw | door | chair | table | bkcase | sofa | board | clutter | **mIOU** | **mAcc** |
|---|---|---|---|---|---|---|---|---|---|---|---|---|---|---|---|
| PointNet [8] | 88.80 | 97.33 | 69.80 | 0.05 | 3.92 | 46.26 | 10.76 | 52.61 | 58.93 | 40.28 | 5.85 | 26.38 | 33.22 | 41.09 | 48.98 |
| SegCloud [13] | 90.06 | 96.05 | 69.86 | 0.00 | 18.37 | 38.35 | 23.12 | 75.89 | 70.40 | 58.42 | 40.88 | 12.96 | 41.60 | 48.92 | 57.35 |
| TangentConv* [12] | 90.47 | 97.66 | 73.99 | 0.0 | 20.66 | 38.98 | 31.34 | 77.49 | 69.43 | 57.27 | 38.54 | 48.78 | 39.79 | 52.8 | 60.7 |
| 3D RNN [15] | 95.2 | 98.6 | 77.4 | 0.8 | 9.83 | 52.7 | 27.9 | 76.8 | 78.3 | 58.6 | 27.4 | 39.1 | 51.0 | 53.4 | 71.3 |
| PointCNN [6] | 92.31 | 98.24 | 79.41 | 0.00 | 17.60 | 22.77 | 62.09 | 80.59 | 74.39 | 66.67 | 31.67 | 62.05 | 56.74 | 57.26 | 63.86 |
| SuperpointGraph [5] | 89.35 | 96.87 | 78.12 | 0.0 | 42.81 | 48.93 | 61.58 | 84.66 | 75.41 | 69.84 | 52.60 | 2.1 | 52.22 | 58.04 | 66.5 |
| PCCN [14] | 90.26 | 96.20 | 75.89 | 0.27 | 5.98 | 69.49 | 63.45 | 66.87 | 65.63 | 47.28 | 68.91 | 59.10 | 46.22 | 58.27 | 67.01 |
| MinkowskiNet20 | 91.55 | 98.49 | 84.99 | 0.8 | 26.47 | 46.18 | 55.82 | 88.99 | 80.52 | 71.74 | 48.29 | 62.98 | 57.72 | 62.60 | 69.62 |
| MinkowskiNet32 | 91.75 | 98.71 | 86.19 | 0.0 | 34.06 | 48.90 | 62.44 | 89.82 | 81.57 | 74.88 | 47.21 | 74.44 | 58.57 | **65.35** | **71.71** |

*Data from the authors

Table 3: Semantic segmentation results on the 4D Synthia dataset

| Method | Bldn | Road | Sdwlk | Fence | Vegittn | Pole | Car | T. Sign | Pedstrn | Bicycl | Lane | T. Light | mIOU | mAcc |
|---|---|---|---|---|---|---|---|---|---|---|---|---|---|---|
| MinkNet20 | 89.394 | 97.684 | 69.425 | 86.519 | 98.106 | 97.256 | 93.497 | 79.450 | 92.274 | 0.000 | 44.609 | 66.691 | 76.24 | 89.31 |
| MinkNet20 + TA | 88.096 | 97.790 | 78.329 | 87.088 | 96.540 | 97.486 | 94.203 | 78.831 | 92.489 | 0.000 | 46.407 | 67.071 | 77.03 | 89.198 |
| 4D MinkNet20 | 90.125 | 98.262 | 73.467 | 87.187 | 99.099 | 97.502 | 94.010 | 79.041 | 92.622 | 0.000 | 50.006 | 68.138 | 77.46 | 88.013 |
| 4D Tesseract MinkNet20 | 89.346 | 97.291 | 60.712 | 86.451 | 98.000 | 96.632 | 93.191 | 74.906 | 91.030 | 0.000 | 47.113 | 69.343 | 75.335 | 89.272 |
| 4D MinkNet20 + TS-CRF | 89.438 | 98.291 | 79.938 | 86.254 | 98.707 | 97.142 | 95.045 | 81.592 | 91.540 | 0.000 | 54.596 | 67.067 | 78.30 | 90.23 |
| 4D MinkNet32 + TS-CRF | 89.694 | 98.632 | 86.893 | 87.801 | 98.776 | 97.284 | 94.039 | 80.292 | 92.300 | 0.000 | 49.299 | 69.060 | **78.67** | **90.51** |

Table 4: Semantic segmentation results on the RueMongue [10] (Varcity) dataset

| Method | window | wall | balcony | door | roof | sky | shop | mIOU |
|---|---|---|---|---|---|---|---|---|
| 3D MinkNet20 | 61.978 | 80.813 | 64.303 | 47.256 | 61.486 | 76.901 | 72.498 | 66.462 |
| 4D MinkNet20 | 61.938 | 81.591 | 65.394 | 35.089 | 68.554 | 80.546 | 72.846 | 66.565 |
| 4D MinkNet20 + TS-CRF | 62.600 | 81.821 | 63.599 | 40.795 | 66.229 | 80.464 | 70.639 | 66.592 |

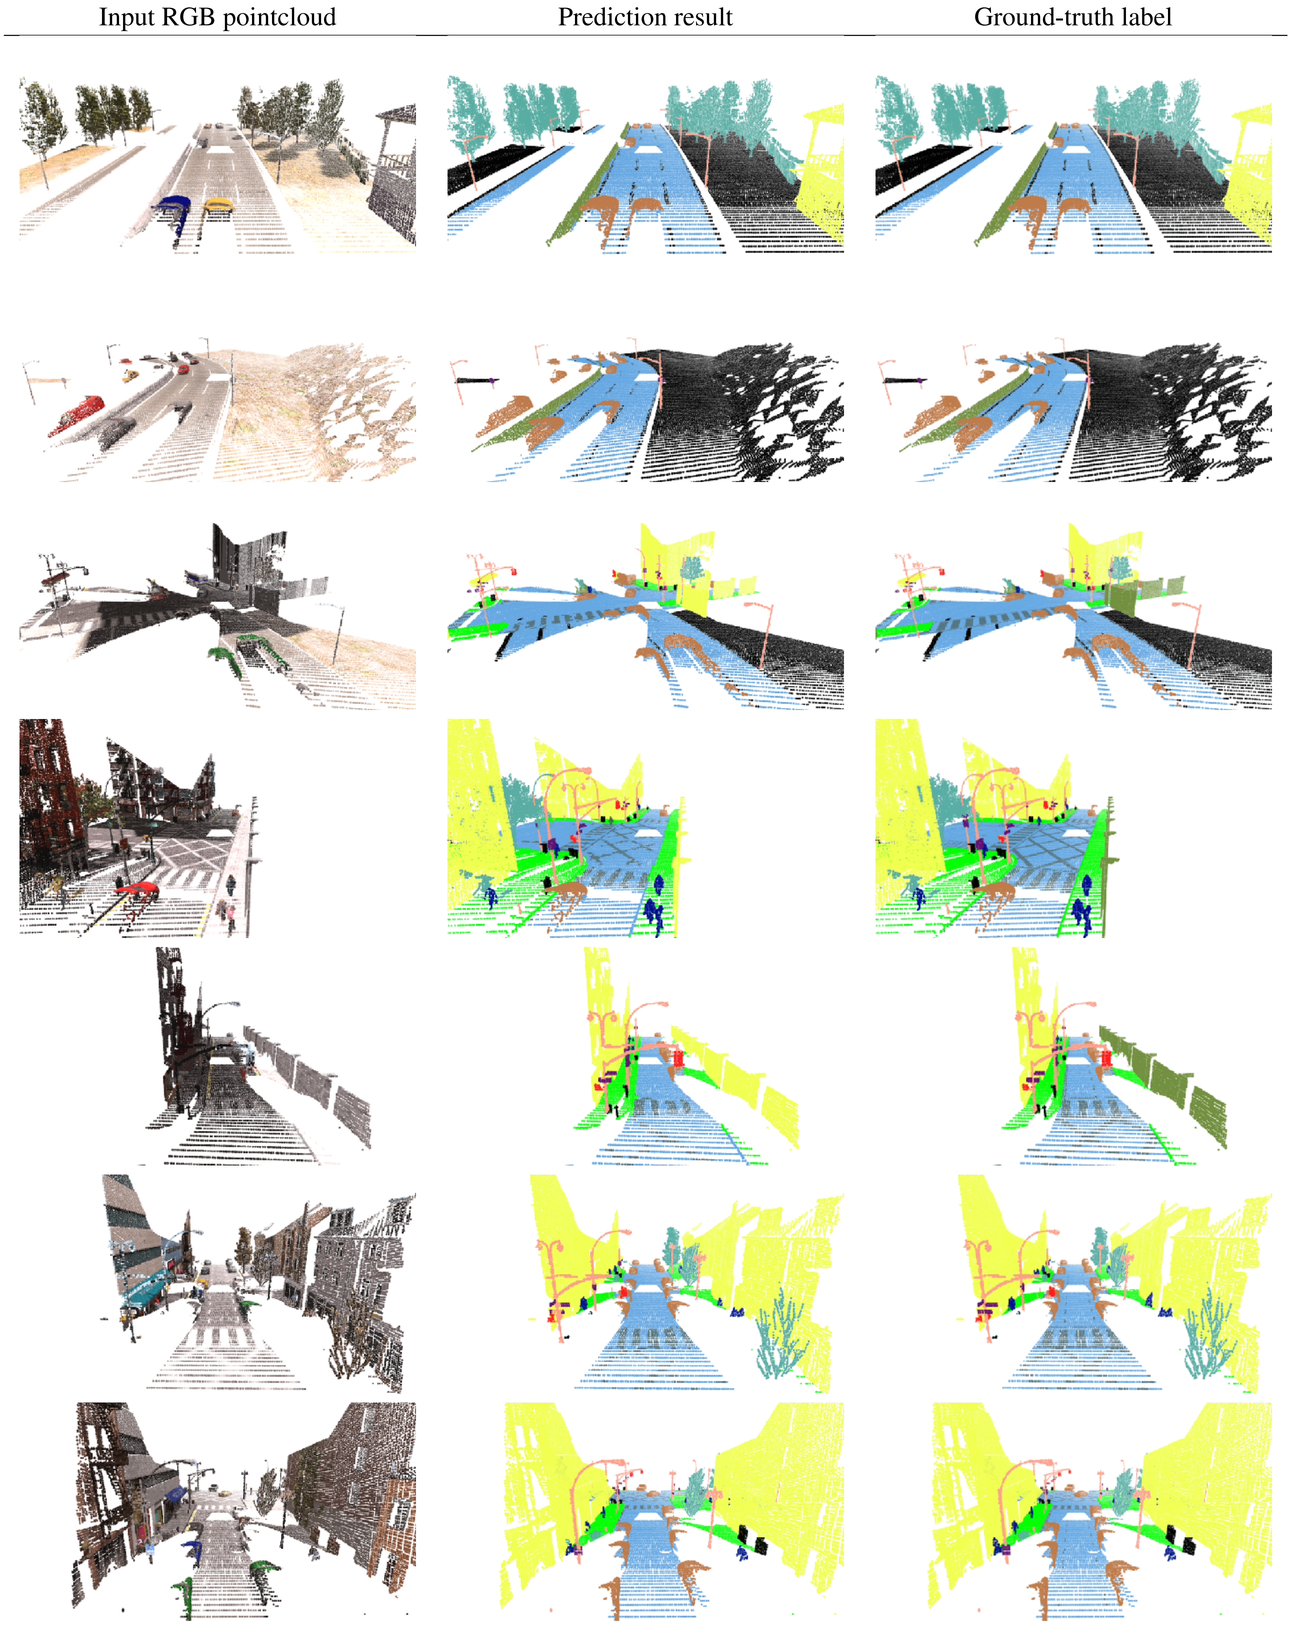


Figure 2: Visualization of the 4D Synthia predictions and ground truth labels.

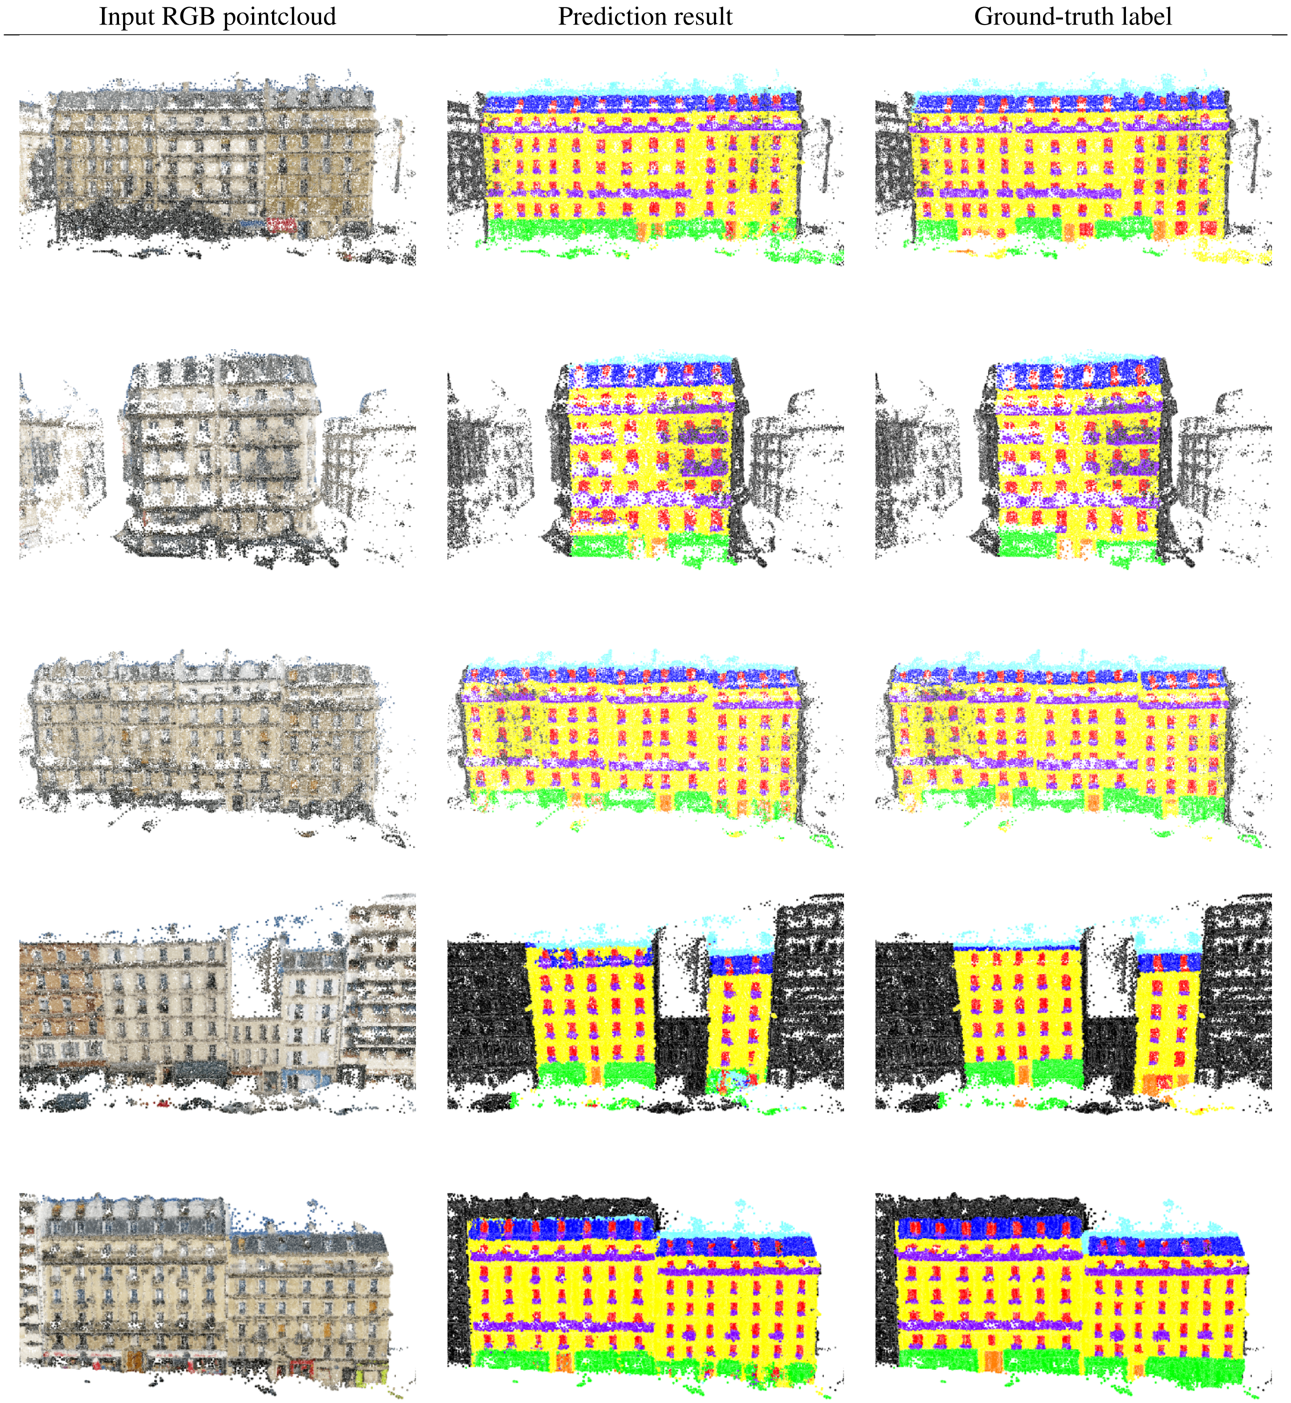


Figure 3: Visualization of the RueMonge 2014 dataset TASK3 results.

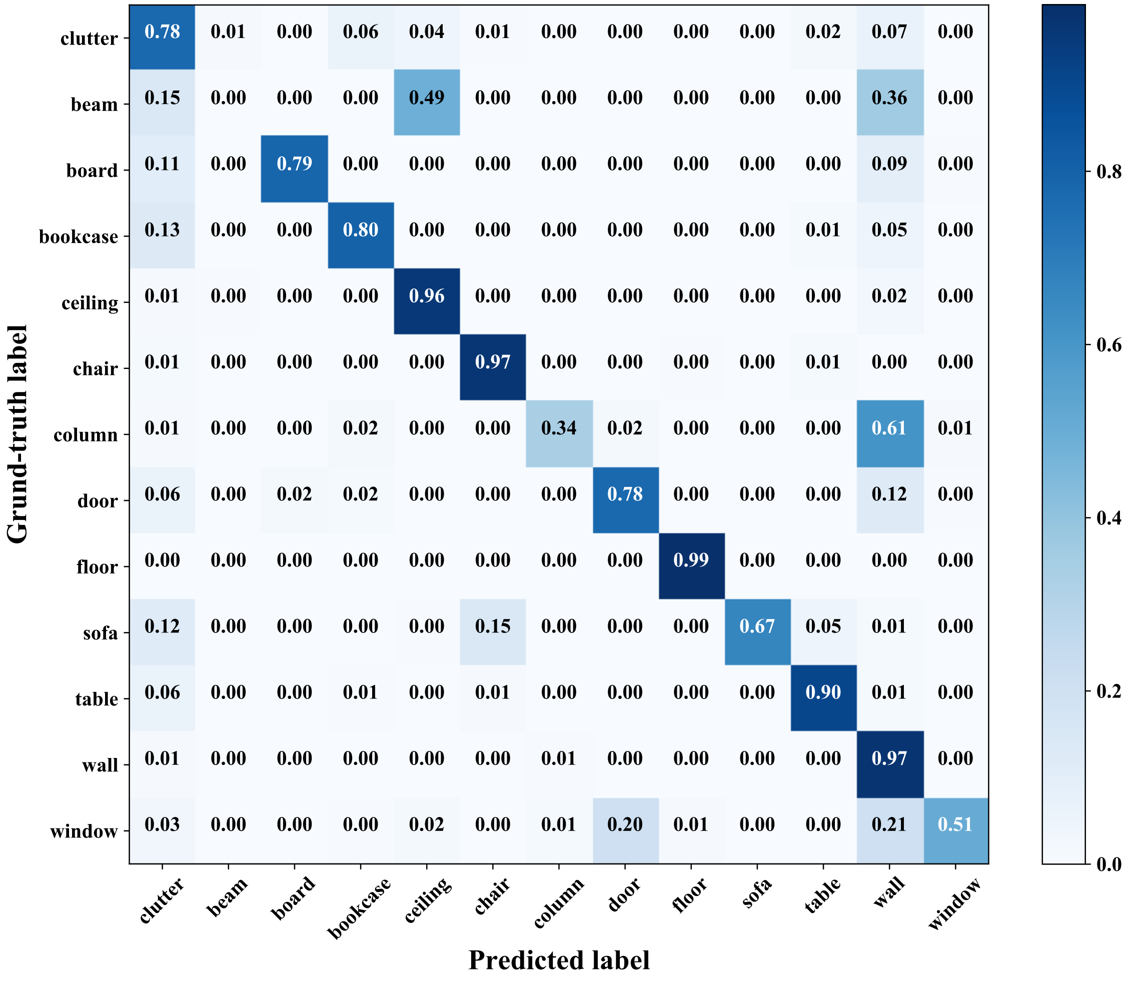


Figure 4: The confusion matrix of the MinkowskiNet32 predictions on the Stanford dataset Area 5 (Fold #1).

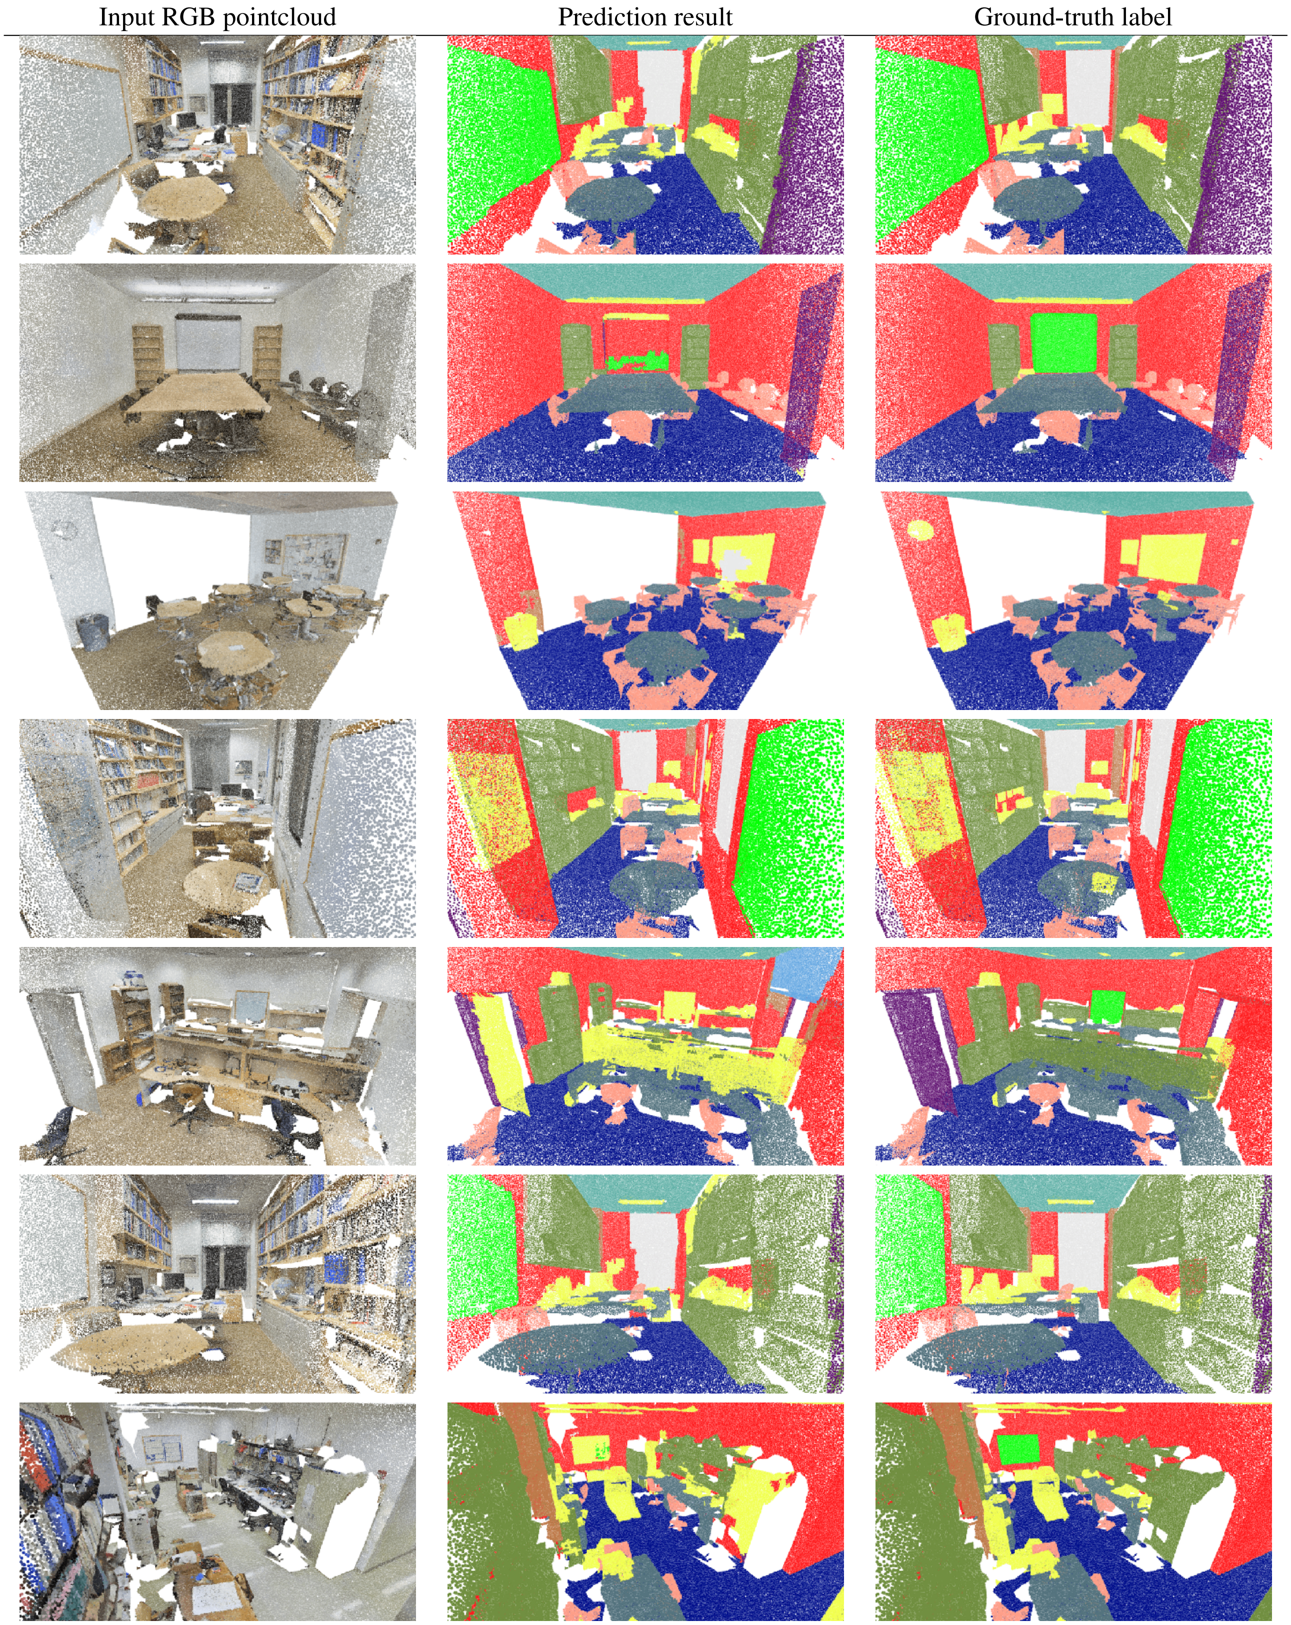


Figure 5: Visualization of the Stanford dataset Area 5 test result.

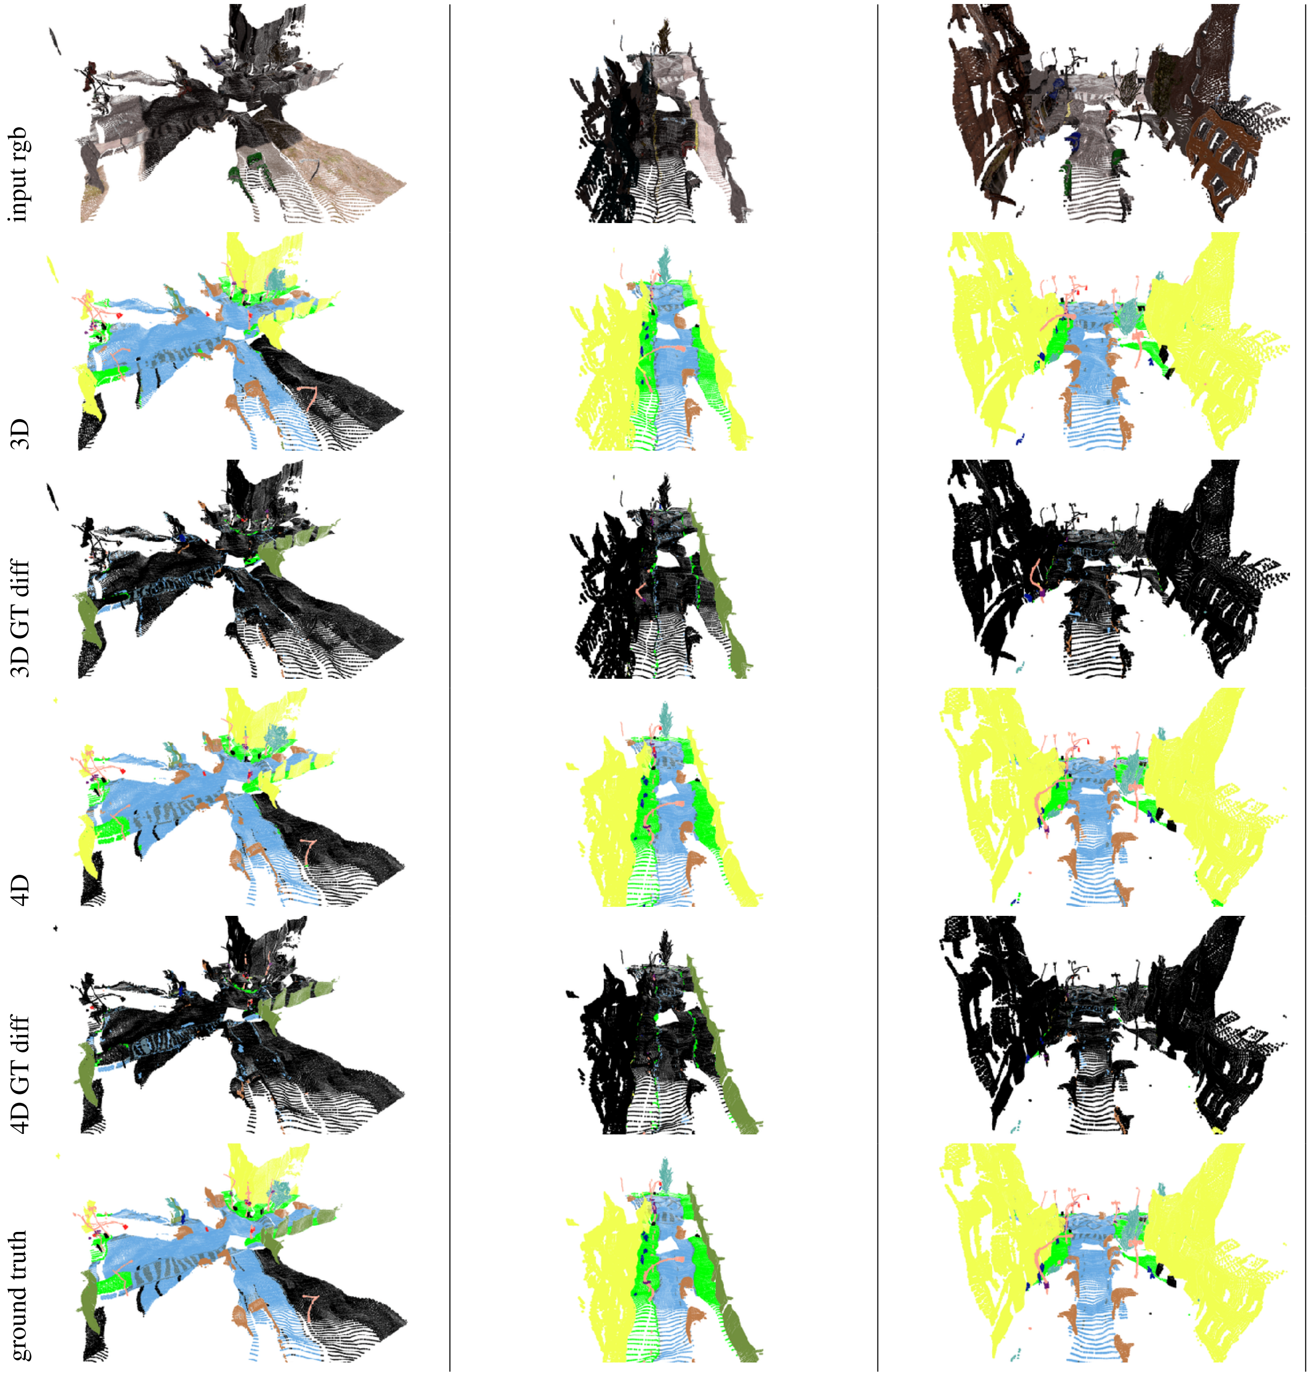


Figure 6: Visualization of the noisy 4D Synthia dataset and predictions.

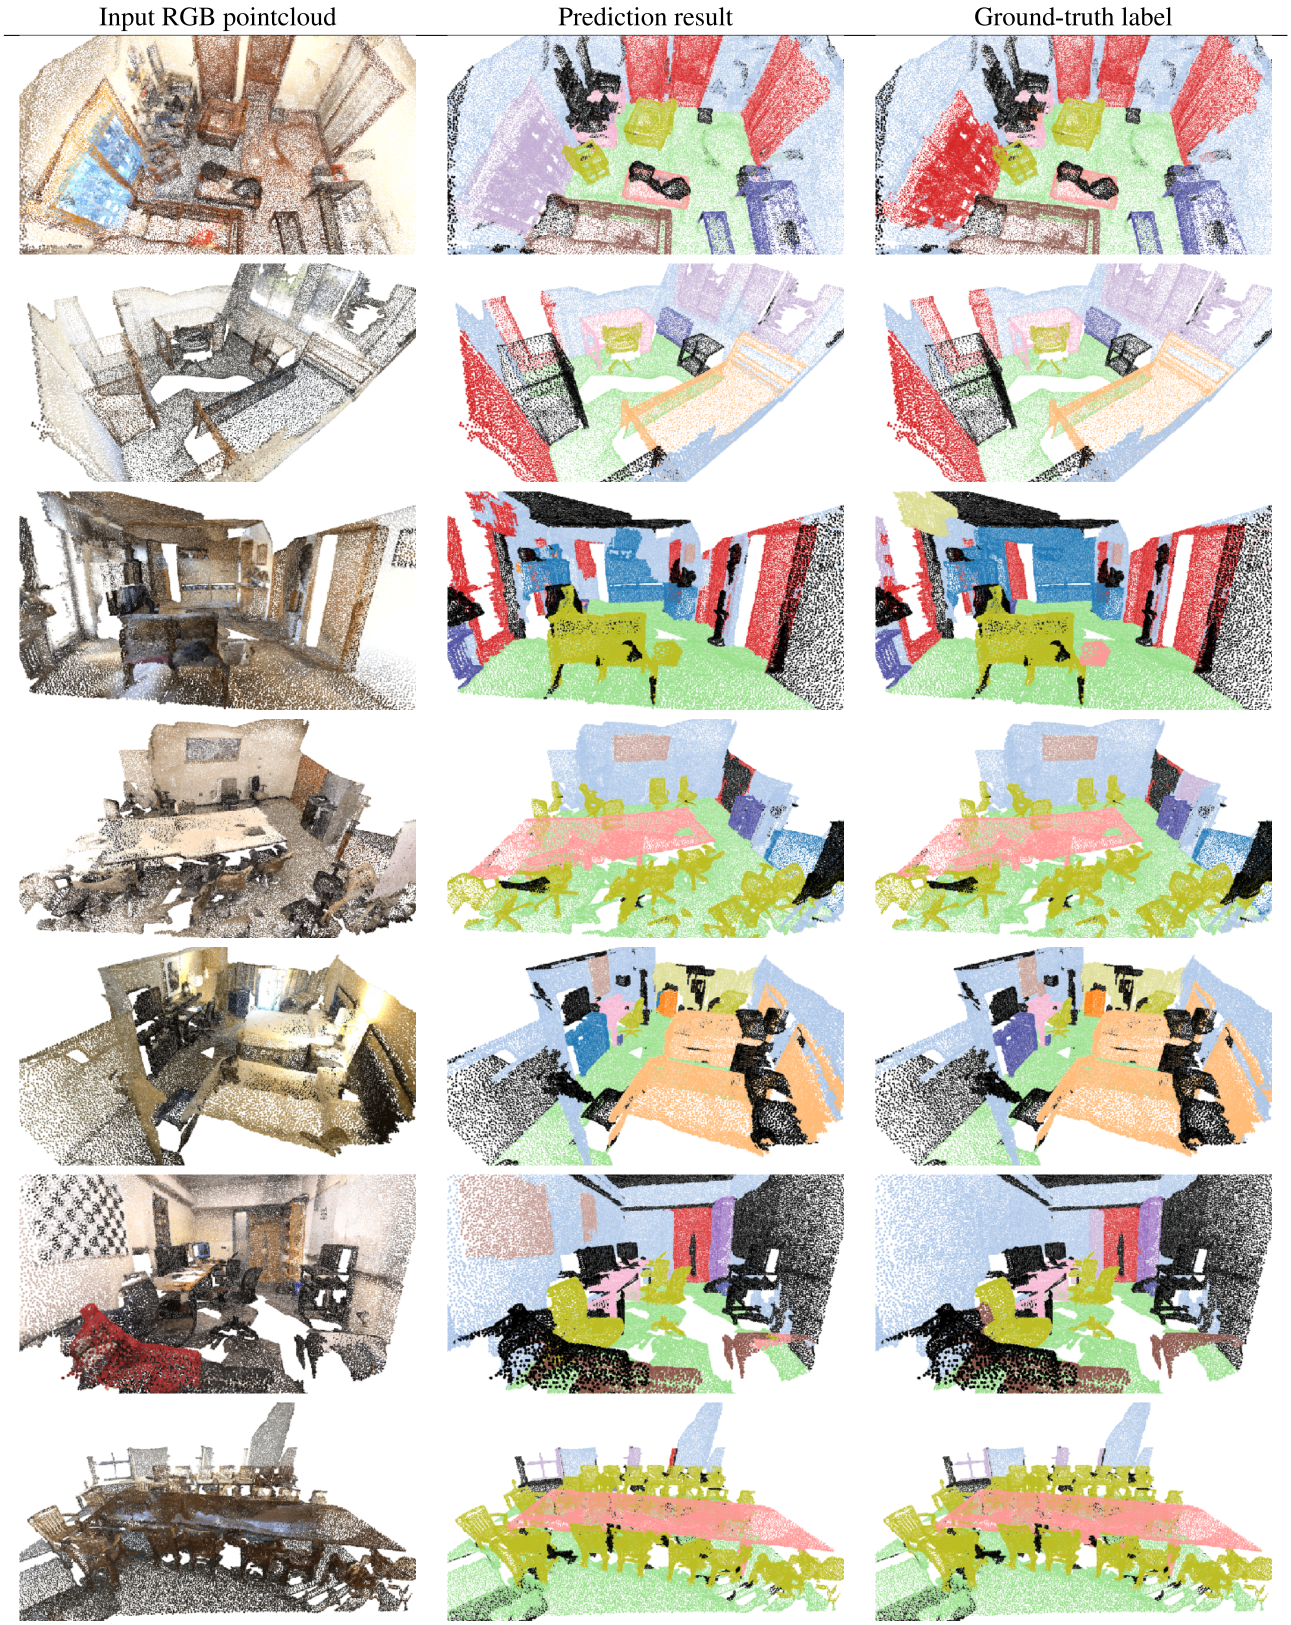


Figure 7: Visualization of MinkNet predictions on the Scannet validation set.

## References


[1] Angela Dai, Angel X. Chang, Manolis Savva, Maciej Halber, Thomas Funkhouser, and Matthias Nießner. Scannet: Richly-annotated 3d reconstructions of indoor scenes. In *Proc. Computer Vision and Pattern Recognition (CVPR), IEEE*, 2017. 3

[2] Angela Dai and Matthias Nießner. 3dmv: Joint 3d-multi-view prediction for 3d semantic scene segmentation. In *Proceedings of the European Conference on Computer Vision (ECCV)*, 2018. 3

[3] Ben Graham. Sparse 3d convolutional neural networks. *British Machine Vision Conference*, 2015. 3

[4] Daphne Koller and Nir Friedman. *Probabilistic Graphical Models: Principles and Techniques - Adaptive Computation and Machine Learning*. The MIT Press, 2009. 2

[5] Loic Landrieu and Martin Simonovsky. Large-scale point cloud semantic segmentation with superpoint graphs. *arXiv preprint arXiv:1711.09869*, 2017. 4

[6] Yangyan Li, Rui Bu, Mingchao Sun, and Baoquan Chen. Pointcnn. *arXiv preprint arXiv:1801.07791*, 2018. 4

[7] Hao Pan, Shilin Liu, Yang Liu, and Xin Tong. Convolutional neural networks on 3d surfaces using parallel frames. *arXiv preprint arXiv:1808.04952*, 2018. 3

[8] Charles Ruizhongtai Qi, Hao Su, Kaichun Mo, and Leonidas J. Guibas. Pointnet: Deep learning on point sets for 3d classification and segmentation. *arXiv preprint arXiv:1612.00593*, 2016. 4

[9] Charles Ruizhongtai Qi, Li Yi, Hao Su, and Leonidas J Guibas. Pointnet++: Deep hierarchical feature learning on point sets in a metric space. In *Advances in Neural Information Processing Systems*, 2017. 3

[10] Hayko Riemenschneider, András Bódis-Szomorú, Julien Weissenberg, and Luc Van Gool. Learning where to classify in multi-view semantic segmentation. In *European Conference on Computer Vision*. Springer, 2014. 4

[11] Hang Su, Varun Jampani, Deqing Sun, Subhransu Maji, Vangelis Kalogerakis, Ming-Hsuan Yang, and Jan Kautz. Splatnet: Sparse lattice networks for point cloud processing. *arXiv preprint arXiv:1802.08275*, 2018. 3

[12] Maxim Tatarchenko*, Jaesik Park*, Vladlen Koltun, and Qian-Yi Zhou. Tangent convolutions for dense prediction in 3D. *CVPR*, 2018. 3, 4

[13] Lyne P Tchapmi, Christopher B Choy, Iro Armeni, JunYoung Gwak, and Silvio Savarese. Segcloud: Semantic segmentation of 3d point clouds. *International Conference on 3D Vision (3DV)*, 2017. 4

[14] Shenlong Wang, Simon Suo, Wei-Chiu Ma3 Andrei Pokrovsky, and Raquel Urtasun. Deep parametric continuous convolutional neural networks. In *Proceedings of the IEEE Conference on Computer Vision and Pattern Recognition*, pages 2589–2597, 2018. 4

[15] Xiaoqing Ye, Jiamao Li, Hexiao Huang, Liang Du, and Xiaolin Zhang. 3d recurrent neural networks with context fusion for point cloud semantic segmentation. In *The European Conference on Computer Vision (ECCV)*, September 2018. 4
